# Supplementary material for: Noninvasive Quantum Measurement of Arbitrary Operator Order by Engineered Non-Markovian Detectors
Source: arXiv:1711.11347 source file (2018-03-08)
Supplement: Supplementary file 1 [file bbbb_SM3.1.pdf]

# Supplemental Material: Noninvasive Quantum Measurement of Arbitrary Operator Order by Engineered Non-Markovian Detectors

Johannes Bülte,[1] Adam Bednorz,[2] Christoph Bruder,[3] and Wolfgang Belzig[1]

[1] *Fachbereich Physik, Universität Konstanz, D-78457 Konstanz, Germany*
[2] *Faculty of Physics, University of Warsaw, ul. Pasteura 5, PL02-093 Warsaw, Poland*
[3] *Department of Physics, University of Basel, Klingelbergstrasse 82, CH-4056 Basel, Switzerland*

(Dated: July 26, 2017)

## SUPPLEMENTAL MATERIAL

### A. Extension of the Model Hamiltonian

To provide maximal clarity we used a simple model Hamiltonian for our calculations. However, it can easily be extended to multiple detectors and more advanced coupling dependencies. The system of interest which we want to measure is denoted by $\hat{H}_0$, the subsystems of the $N$ detectors which are coupled to the system of interest are labeled by $i = 1, 2, 3, \ldots, N$, so that the total Hamiltonian is given by

$$\hat{H} = \sum_{i=0}^{N} \hat{H}_i + \hat{H}_{\mathrm{int}}, \tag{1}$$

with

$$\hat{H}_{\mathrm{int}}(t) = \sum_{i=1}^{N} \eta_i \Gamma_i(t, \{t_i\}) \int \mathrm{d}\lambda\, \Phi_i(\lambda) \hat{D}_{i,\lambda} \hat{A}_i\, . \tag{2}$$

This is the most general form with the system variables $\hat{A}_i$ coupled to the detector variables $\hat{D}_i$. It contains arbitrary coupling functions $\Gamma_i$ which may depend on the time $t$ and the set of the measurement times of the $N$ different detectors $\{t_i\}$. The cases discussed in the paper are a constant coupling $\Gamma_i = 1$ and a instantaneous/Markovian coupling $\Gamma_i = \delta(t - t_i)$. If a "natural decoupling" of the detector via collapse of its noise in the readout procedure does not occur, it can be imposed by choosing $\Gamma_i \propto \theta(t_i - t)$. Other possibilities are a Gaussian shape or adiabatic coupling. We also introduced the generalization of the detector subsystems to a set of independent detectors distributed over a characteristic parameter $\lambda$ by the density functions $\Phi_i(\lambda)$. This can be a bath of harmonic oscillators, i.e. the parameter is the frequency $\lambda \to \omega$ with the distribution $\Phi(\omega)$. We can incorporate these features in the model discussed in the paper by setting $\hat{D}_i \to \int \mathrm{d}\lambda\, \Phi_i(\lambda) \hat{D}_{i,\lambda}$. Therefore our model covers a variety of systems as long as they fulfill the main constraints (a) weak coupling and (b) linear coupling in system and detector variable.

### B. On the readout of the detector: the post-readout expectation value

An important property of the detector noise terms $C_\alpha^{\mathrm{det}}$ is, that the detector is also a quantum object and the final results will depend on its initial state $\hat{\rho}_d$ and the readout procedure via $\hat{K}_m$. The detector noise for a readout at time $t_m$ in its most general form is given by

$$S_{MD}(t_m, t') = \theta(t_m - t') \mathrm{Tr} \left\{ \{\delta \hat{M}(t_m), \hat{D}(t')\} \hat{\rho}_d \right\} /2 + \theta(t' - t_m) \int \mathrm{d}m\, (m - \langle \hat{M}(t_m) \rangle) \mathrm{Tr} \left\{ \hat{D}(t') \hat{K}_m(t_m) \hat{\rho}_d \hat{K}_m^\dagger(t_m) \right\}\, . \tag{3}$$

We illustrate some of the possible outcomes with the example of a harmonic oscillator $\hat{H} = \hbar\Omega \left( \hat{a}^\dagger \hat{a} + \frac{1}{2} \right)$.

If we choose $\hat{M} = \hat{x}$ and $\hat{D} = \hat{p}$ and perform a projective detector readout $\hat{K}_x = |x\rangle\langle x|$ we find in a (stationary) thermal initial state as well as in a (non-stationary) coherent intial state that the state does not change due to the readout. It is a non-demolition measurement.

If we choose $\hat{M} = \hat{a}^\dagger \hat{a} = \hat{n}$ and $\hat{D} = \hat{a} + \hat{a}^\dagger$ the noise is given by

$$\begin{aligned} S_{MD}(t_m, t') =& \theta(t_m - t') \mathrm{Tr} \left\{ \{\hat{a}^\dagger \hat{a}, \hat{a} e^{-i\Omega t'} + \hat{a}^{\dagger e^{i\Omega t'}} \} \hat{\rho}_d \right\} /2 - \mathrm{Tr} \left\{ \hat{a}^\dagger \hat{a} \hat{\rho}_d \right\} \mathrm{Tr} \left\{ \hat{a} e^{-i\Omega t'} + \hat{a}^\dagger e^{i\Omega t'} \hat{\rho}_d \right\} \\ &+ \theta(t' - t_m) \int \mathrm{d}n\, (n - \langle \hat{n}(t) \rangle) \mathrm{Tr} \left\{ (\hat{a}(t') + \hat{a}^\dagger(t')) \hat{K}_n(t) \hat{\rho}_d \hat{K}_n^\dagger(t) \right\}\, . \end{aligned} \tag{4}$$

In a coherent state and with a projective readout $\hat{K}_n = |n\rangle\langle n|$ the result is $S_{MD}(t_m, t') = \theta(t_m - t')\mathrm{Re}\left\{\alpha e^{-i\Omega t'}\right\}$ because the term after the readout vanishes $\int \mathrm{d}n\, \mathrm{Tr}\left\{(n - \langle\hat{n}(t)\rangle)|n\rangle\langle n|(\hat{a}(t') + \hat{a}^\dagger(t'))|n\rangle\langle n|\hat{\rho}_d\right\} = 0$ due to $\langle n|(\hat{a}(t') + \hat{a}^\dagger(t'))|n\rangle = 0$. Therefore we get no post-readout noise contribution and find a natural decoupling of the detector.

In general we can state that a self-decoupling detector requires no non-zero diagonal elements of $\hat{D}$ in the eigenbasis of $\hat{M}$: $D_{mm}(t) = 0\ \forall\, m, t$. The resulting vanishing noise is determined already by the choice of the detector variables and is independent of the state of the detector. Alternatively, we obtain vanishing noise after the readout if the detector state is chosen such that there is exactly one non-zero element of $\hat{\rho}_d$ in the eigenbasis of $\hat{M}$: $\rho_{d,mm}(t) = \begin{cases} 0 \text{ if } m \neq m'(t) \\ 1 \text{ if } m = m'(t) \end{cases}$ $\forall t$. Due to $\langle\hat{M}(t)\rangle = m'$ the post-readout noise equals zero. If $\hat{\rho}_d$ represents a pure eigenstate of $\hat{M}$ the response $\chi_{MD}$ will also vanish because the expectation value of the commutator equals to zero. Anyhow, if there are coherent parts in $\hat{\rho}_d$ a finite response $\chi_{MD}$ occurs.

### C. The dependence of the detector observable on the readout

The general form of the detector observable is given by $\hat{M}_\alpha = \int \mathrm{d}m_\alpha\, m_\alpha \hat{K}^\dagger_{m_\alpha}\hat{K}_{m_\alpha}$. In the examples in our work we have chosen the form which it gets from a projective readout $\hat{M}_\alpha = \int \mathrm{d}m_\alpha\, m_\alpha |m_\alpha\rangle\langle m_\alpha|$. Here we show that for an noninvasive readout of the detector we can still have $\hat{M}_\alpha \propto \int \mathrm{d}m_\alpha\, m_\alpha|m_\alpha\rangle\langle m_\alpha|$ with a scalar proportionality constant which can easily be absorbed in the coupling parameters $\eta_\alpha$.

We consider an example with a readout system with Hilbert space $\mathcal{H}_R$ coupled to our detector system $\mathcal{H}_D$. The readout system is initialized with a pointer wave function $|\psi\rangle$, its momentum couples instantaneously to the detector variable $\hat{M}$ so that the time evolution in the interaction picture is given by $\hat{U}_I = e^{-i\xi\hat{M}\hat{p}}$ with a small coupling parameter $\xi$. After the interaction the position in the readout system is measured. The Kraus operator for finding the result $x$ is given by

$$\hat{K}_x = \langle x|\hat{U}_I|\psi\rangle\ . \tag{5}$$

With the spectral representation $\sum_m m|m\rangle\langle m|$ the interaction can be written as

$$\hat{U}_I = \sum_m e^{-i\xi m\hat{p}}|m\rangle\langle m|, \tag{6}$$

so that we obtain

$$\hat{K}_x = \sum_m \psi(x + \xi m)|m\rangle\langle m|\ . \tag{7}$$

If we now assume weak coupling and expand the wavefunction $\psi$ to first order in $\xi$ we get

$$\hat{K}_x = \psi(x)\hat{1} + \xi\psi'(x)\hat{M}\ . \tag{8}$$

This implies

$$\hat{K}^\dagger_x\hat{K}_x = |\psi(x)|^2\hat{1} + \xi(\psi'(x)\psi^*(x) + \psi'^*(x)\psi(x))\sum_m m|m\rangle\langle m| + O(\xi^2)\ , \tag{9}$$

which satisfies $\int \mathrm{d}x\, \hat{K}^\dagger_x\hat{K}_x = \hat{1}$ if the detector is calibrated with $\langle x\rangle = 0$. The measured operator is

$$\hat{M} = \int \mathrm{d}x\, x\hat{K}^\dagger_x\hat{K}_x = \xi\int \mathrm{d}x\, x(\psi'(x)\psi^*(x) + \psi'^*(x)\psi(x))\sum_m m|m\rangle\langle m|\ . \tag{10}$$

Therefore, with the weak detector measurement we obtain $\hat{M} = \zeta\sum_m m|m\rangle\langle m|$ and the result is only changed by a scalar factor which depends exclusively on the readout system

$$\zeta = \xi\int \mathrm{d}x\, x(\psi'(x)\psi^*(x) + \psi'^*(x)\psi(x))\ . \tag{11}$$

### D. Damping of the harmonic oscillator detector

Without damping the response and noise functions of a harmonic oscillator detector (frequency $\Omega'$, ladder operators $\hat{a}$) with the choice $\hat{M} = \hat{x}$ and $\hat{D} = \hat{p}$ are given by

$$\chi_{MD}(t) = \theta(t)\cos(\Omega' t), \tag{12}$$

and

$$S_{MD}(t) \;=\; \sin(\Omega' t)\coth(\beta\Omega'/2)/2, \tag{13}$$

where $\beta$ is the detector's inverse temperature.

We model damping by coupling the detector-oscillator to a bath of harmonic oscillators (ladder operators $\hat{b}_j$). This can be traced out and leads to effective dissipation. We add the reservoir by

$$H_{\mathrm{bath}} = \sum_j \omega_j \hat{b}_j^\dagger \hat{b}_j, \tag{14}$$

and couple it to the detector-oscillator with

$$H_{\text{det-bath}} = \sum_j \xi_j \hat{a}^\dagger \hat{b}_j + \xi_j^* \hat{a}\hat{b}_j^\dagger. \tag{15}$$

The Heisenberg equations of motion read

$$\frac{\mathrm{d}}{\mathrm{d}t}\hat{a}(t) = -i\Omega'\hat{a}(t) - i\sum_j \xi_j \hat{b}_j(t),\; \frac{\mathrm{d}}{\mathrm{d}t}\hat{b}_j(t) = -i\omega_j\hat{b}_j(t) - i\xi_j^*\hat{a}(t)\,. \tag{16}$$

Plugging the solution of the second equation, $\hat{b}_j(t) = e^{-i\omega_j t}\hat{b}_j - i\xi_j^*\int_0^t \mathrm{d}t' e^{i\omega_j(t'-t)}\hat{a}(t')$, into the first one, we obtain

$$\frac{\mathrm{d}}{\mathrm{d}t}\hat{a}(t) = -\sum_j |\xi_j|^2 \int_0^t \mathrm{d}t' e^{-i\omega_j t'}\hat{a}(t-t') - i\Omega'\hat{a}(t) + \hat{F}(t), \tag{17}$$

with $\hat{F}(t) = -i\sum_j \xi_j \hat{b}_j e^{-i\omega_j t}$. The first term can be approximated as $-\lambda\hat{a}(t)$ with

$$\lambda = \int_0^\infty \sum_j |\xi_j|^2 e^{-i(\omega_j - \Omega')t}\mathrm{d}t = \sum_j \frac{|\xi_j^2|}{i(\omega_j - \Omega') + 0_+}, \tag{18}$$

if $\xi$ changes much more slowly with $j$ than $\omega$. This leads to the Langevin equation

$$\frac{\mathrm{d}}{\mathrm{d}t}\hat{a}(t) = -(\lambda + i\Omega')\hat{a}(t) + \hat{F}(t), \tag{19}$$

that is solved by

$$\hat{a}(t) = e^{-(\lambda+i\Omega')(t-t_0)}\left(\hat{a} + \int_{t_0}^t e^{(\lambda+i\Omega')(t'-t_0)}\hat{F}(t')\mathrm{d}t'\right). \tag{20}$$

If we trace out the bath, due to

$$\mathrm{Tr}_{\mathrm{bath}}\hat{F}(t) = -i\sum_j \xi_j \mathrm{Tr}_{\mathrm{bath}}(\hat{b}_j)e^{-i\omega_j t} = 0\,, \tag{21}$$

the only remaining modification is a damping factor $\lambda$ in the exponentials:

$$\chi_{MD}(t) = \theta(t)e^{-\lambda t}\cos(\Omega' t), \tag{22}$$

and

$$S_{MD}(t) \;=\; e^{-\lambda t}\sin(\Omega' t)\coth(\beta\Omega'/2)/2\,. \tag{23}$$

### E. Extracting different operator orders from a noise measurement

If system and detectors are initialized in stationary states we can write in Fourier space

$$\begin{aligned}C(\omega) =&\chi^a_{MD}(\omega)\chi^b_{MD}(-\omega)S^0_{AB}(\omega)\\&+\chi^b_{MD}(-\omega)\chi^0_{BA}(-\omega)S^a_{MD}(\omega)\\&+\chi^a_{MD}(\omega)\chi^0_{AB}(\omega)S^b_{MD}(-\omega).\end{aligned} \tag{24}$$

We consider two thermal detectors of the same type, for which the fluctuation-dissipation theorem and causality imply

$$C(\omega) =i\coth(\beta_d\omega/2)\chi_{MD}(\omega)-2i\int\frac{\mathrm{d}\omega'}{2\pi}\frac{\tanh(\beta_d\omega'/2)}{\tanh(\beta_d\omega/2)}\frac{S_{MD}(\omega')}{\omega-\omega'}, \tag{25}$$

and investigate two different coupling cases for the detector

$$S^{\mathrm{P}}_{MD}(\omega)=\begin{cases}S_{MD}(\omega) & \text{persistent coupling}\\ \frac{S_{MD}(\omega)}{2}+i\int\frac{\mathrm{d}\omega'}{2\pi}\frac{S_{MD}(\omega')}{\omega-\omega'} & \text{decoupling.}\end{cases} \tag{26}$$

*Noninvasive detector readout / persistent coupling* — This case is relevant for a noninvasive readout, e.g. a weak measurement of the detector, "classical readout" or a non-demolition quantum measurement on the detector. With the notation $\chi_{XY}(\omega)=\chi^{(1)}_{XY}(\omega)+\chi^{(2)}_{XY}(\omega)$, where $\chi^{(1)}_{XY}(\omega)=\tilde{\chi}_{XY}(\omega)/2$ and $\chi^{(2)}_{XY}(\omega)=i\int\frac{\mathrm{d}\omega'}{2\pi}\frac{\tilde{\chi}_{XY}(\omega')}{\omega-\omega'}$ we can write

$$\begin{aligned}C(\omega)=&|\chi_{M,D}(\omega)|^2\left(S_{AB}(\omega)-2i\coth(\beta_d\omega/2)\chi^{(1)}_{A,B}(\omega)\right)\\&+2i\coth(\beta_d\omega/2)\left[\chi^{(1)}_{A,B}(\omega)\chi^{(2)}_{M,D}(\omega)+\chi^{(2)}_{A,B}(\omega)\chi^{(1)}_{M,D}(\omega)\right]\chi^{(2)}_{M,D}(\omega)\,.\end{aligned} \tag{27}$$

In this discussion, $\tilde{\chi}_{MD}(\omega)=\int\mathrm{d}t\,e^{i\omega t}\langle[\hat{M}(t),\hat{D}]\rangle$ is assumed to be real. For a broadband detector $\chi_{MD}(\omega)=1$ we obtain

$$C(\omega)=S_{AB}(\omega)-2i\coth(\beta_d\omega/2)\chi^{(1)}_{A,B}(\omega). \tag{28}$$

In a thermal state it is $\chi^{(1)}_{A,B}(\omega)=-i\tanh(\beta_s\omega/2)S_{AB}(\omega)$ and at $\beta_d=\beta_s$ the system noise term and the two detector noise terms contribute in equal parts to the total noise.

If the detector temperature is tunable without affecting the system (much), the different system operator orders can be extracted from a series of two noise measurements. The system is herein allowed to be in an arbitrary quantum state. The weight of the antisymmetric system term is tuned by the detector temperature and can therefore be separated if we perform two measurements at two different detector temperatures $C(\omega)|_{\beta_{d,1}}$ and $C(\omega)|_{\beta_{d,2}\neq\beta_{d,1}}$.

*Invasive detector measurement / decoupling.* — This case is relevant for either a decoupling of the detector due to its vanishing noise after the readout procedure (see Sec. B) or for manual decoupling by engineering a coupling function $\Gamma(t>t_{a,b})=0$.

The detector noise terms in the results previously discussed are halved and we obtain additional terms

$$C^{\mathrm{add}}(\omega)=2i\left[\chi^{(1)}_{MD}(\omega)\chi^{(2)}_{AB}(\omega)+\chi^{(2)}_{MD}(\omega)\chi^{(1)}_{AB}(\omega)\right]\int\frac{\mathrm{d}\omega'}{2\pi}\frac{S_{MD}(\omega')}{\omega-\omega'}. \tag{29}$$

For the broadband detector the total result is given by

$$C(\omega)=S_{AB}(\omega)-i\coth(\beta_d\omega/2)\chi^{(1)}_{AB}(\omega)-2\chi^{(2)}_{AB}(\omega)\int\frac{\mathrm{d}\omega'}{2\pi}\frac{\coth(\beta_d\omega'/2)}{\omega-\omega'}. \tag{30}$$

The first two terms cancel for a system in a thermal state at detector temperature. The last term is a correction to this "equilibrium order". Its relevance depends on the second part of the system's response $\chi^{(2)}_{AB}(\omega)$.

### F. Proposal for a general correlator of weak measurements

A general correlator of weak quantum measurements including nonsymmetric contributions and allowing for finite interaction time of the detector and the system has been developed in [1] by relating the recorded time-dependent signals $a_j(t)$ to a superoperator of the form

$$\check{A}_j^{t-t'}(t') = g_j(t-t')\check{A}_j^c(t') + f_j(t-t')\check{A}_j^q(t')/2. \tag{31}$$

The result reads

$$\langle a_1(t_1)\dots a_n(t_n)\rangle_w = \mathrm{Tr}\left\{\int \mathrm{d}^n t'\, \mathcal{T}[\check{A}_n^{t_n-t'_n}(t'_n)\dots \check{A}_1^{t_1-t'_1}(t'_1)]\hat{\rho}\right\}. \tag{32}$$

Causality is preserved by time ordering and the requirement $g(t<0)=0$. The second-order expression is given by

$$\begin{aligned}\langle a(t_a)b(t_b)\rangle_w =& \int \mathrm{d}t' \int \mathrm{d}s'\, g_1(t_a,t')g_2(t_b,s')\langle\{\hat{A}(t'),\hat{B}(s')\}\rangle/2\\ &- i\int \mathrm{d}t' \int \mathrm{d}s'\, \theta(t'-s')g_1(t_a,t')f_2(t_b,s')\langle[\hat{A}(t'),\hat{B}(s')]\rangle/2\\ &- i\int \mathrm{d}t' \int \mathrm{d}s'\, \theta(s'-t')f_1(t_a,t')g_2(t_b,s')\langle[\hat{B}(s'),\hat{A}(t')]\rangle/2.\end{aligned} \tag{33}$$

The memory functions $f$ and $g$ are determined phenomenologically in this scheme [1] by assuming no frequency filter effect of the detector $g(t)=\delta(t)$ and based on the assumption of a vanishing noise spectral density in thermal equilibrium ($\hat{\rho}_i = e^{-\beta\hat{H}_i}/\mathrm{Tr}\{e^{-\beta\hat{H}_i}\}$)

$$S_{ab}(\omega) = \int \mathrm{d}t\, e^{i\omega t}\langle a(t)b(0)\rangle_w \stackrel{!}{=} 0\,. \tag{34}$$

The functions derived from this condition are denoted as "equilibrium order". By identifying $\langle a(t_a)b(t_b)\rangle_w = C(t_a,t_b)$ we are able to provide microscopic expressions for $f$ and $g$ here. By comparison of both frameworks we find

$$g_\alpha(t,t') = \chi^\alpha_{MD}(t,t'), \tag{35}$$

and

$$f_\alpha(t,t') = 2S^\alpha_{MD}(t,t'). \tag{36}$$

Thus, our new approach provides explicit expressions for $f_\alpha$ and $g_\alpha$ and goes beyond the phenomenological thermal detector approach considered so far.

Among the examples discussed in the present work we explore regimes beyond "equilibrium order" with nonthermal detector and system states and the effect of a quantum readout of the detector. By the identification of the memory functions with the detectors noise and response functions, our microscopic approach can be readily applied to higher-order correlation functions.

[1] A. Bednorz, C. Bruder, B. Reulet and W. Belzig, Phys. Rev. Lett. **110**, 250404 (2013).
